# Supplementary material for: EVQAScore: A Fine-grained Metric for Video Question Answering Data Quality Evaluation
Source: arXiv:2411.06908 source file (2025-02-06)
Supplement: Supplementary file 1 [file X_suppl.tex]

\setcounter{page}{1}
\maketitlesupplementary
\section{Keywords Extraction Prompt}
\begin{figure}[ht]
  \includegraphics[width=0.47\textwidth]{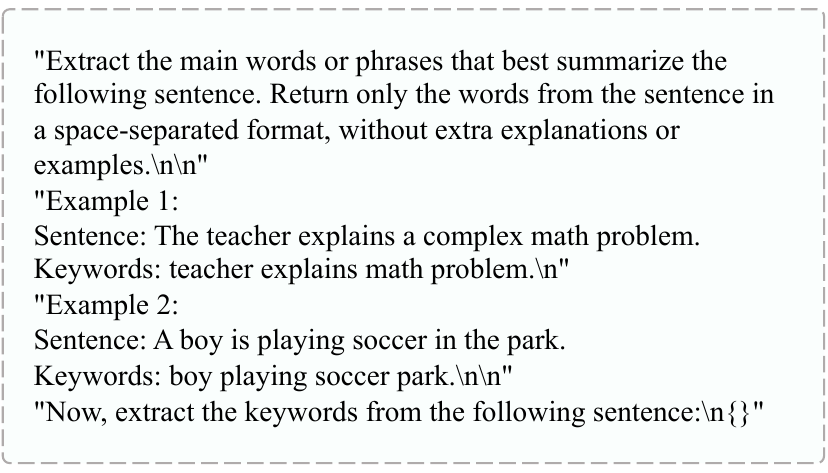}
  \caption{We provide the prompt used for keywords extraction}
  \label{fig:Keywords}
\end{figure}
